# Supplementary material for: Advancements in Traffic Processing Using Programmable Hardware Flow Offload
Source: arXiv:2407.16231 source file (2024-07-23)
Supplement: Supplementary file 1 [file additional.tex]

\bibitem{b1} M. Sheeraz, H. Durad, S. Tahir, H. Tahir, S. Saeed, A.M. Almuhaideb,
``Advancing Snort IPS to Achieve Line Rate Traffic Processing for Effective Network Security Monitoring'',
IEEE Access, 2024.

\bibitem{b2} Q. Zhang, N. Ansari, Z. Zhu,
``Adaptive SmartNIC Offloading for Unleashing the Performance of Protocol-Oblivious Forwarding'',
IEEE Internet of Things Journal, 2022.

\bibitem{b4} S. Panda, et al., ``SmartWatch: Accurate traffic analysis and flow-state tracking for intrusion prevention using SmartNICs'', Proceedings of the 17th International Conference on Emerging Networking, 2021.

\bibitem{b7} C.E. Leiserson, N.C. Thompson, J.S. Emer, B.C. Kuszmaul, B.W. Lampson, D. Sanchez,
``There's plenty of room at the Top: What will drive computer performance after Moore's law?'',
Science, 2020

\bibitem{b8} Dally, William J., Yatish Turakhia, and Song Han,
``Domain-specific hardware accelerators'',
Communications of the ACM 63.7, 2020

\bibitem{b9} Hanford, Nathan, et al,
``A survey of end-system optimizations for high-speed networks'',
ACM Computing Surveys (CSUR) 51.3, 2018

\bibitem{b10} Y. Le, H. Chang, S. Mukherjee, L. Wang, A. Akella, M.M. Swift, T.V. Lakshman,
``UNO: Uniflying host and smart NIC offload for flexible packet processing'',
Proceedings of the 2017 Symposium on Cloud Computing, 2017

\bibitem{b11} P. Rygielski, M. Seliuchenko, S. Kounev, M. Klymash,
``Performance Analysis of SDN Switches with Hardware and Software Flow Tables'',
VALUETOOLS, 2016

\bibitem{b12} D. Vodák, K. Vojanec, J. Šuráň,
``What RTE flow rules can your NIC offload?'',
DPDK Userspace Summit, 2022
